# Supplementary material for: ScreenAgent: A Vision Language Model-driven Computer Control Agent
Source: arXiv:2402.07945 source file (2024-02-09)
Supplement: Supplementary file 1 [file appendix_coco_example.pdf]

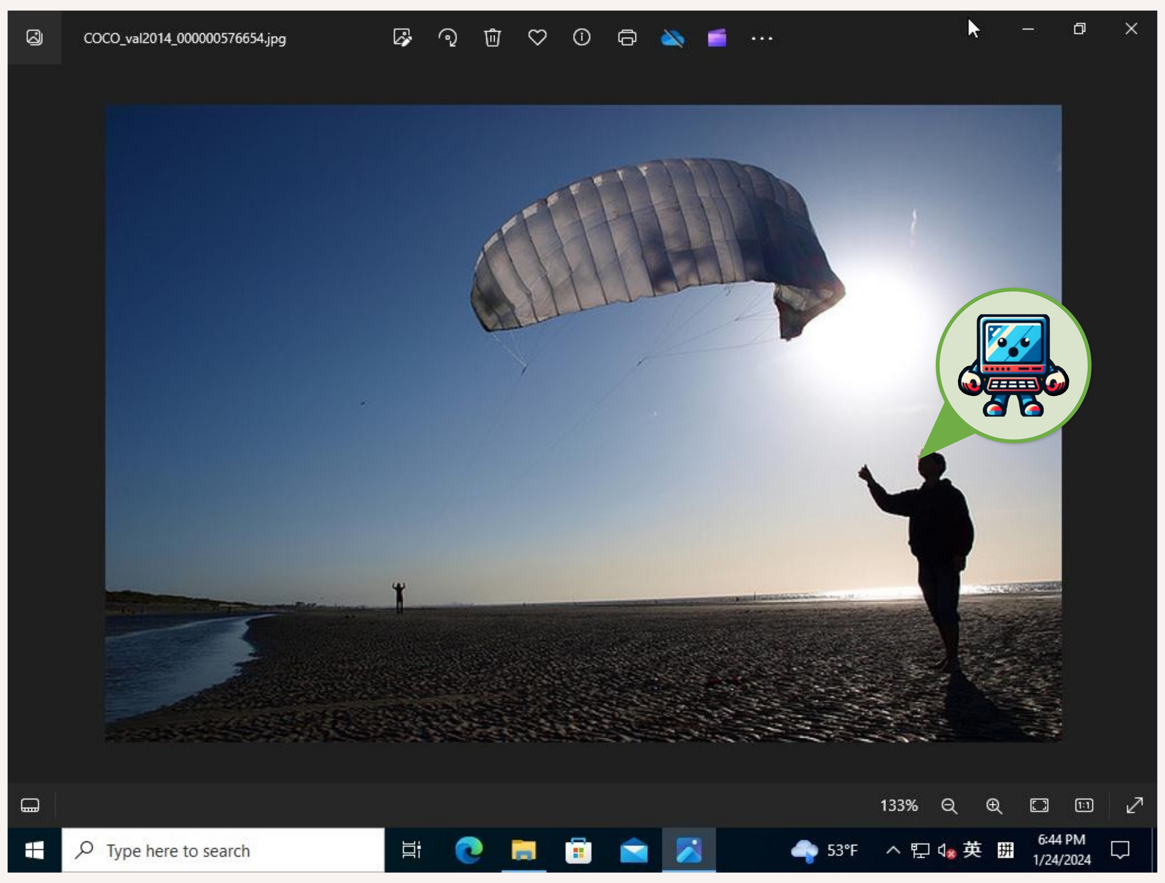


**Subtask:** Click the people in the picture

**ScreenAgent(Acting Phase):**
To complete the subtask "Click the people in the picture", I need to move the mouse cursor to the position of the people in the picture and click.
```json
[
  {"action_type":"MouseAction", "mouse_action_type":"click",
"mouse_button":"left", "mouse_position":{"width":811,"height":400}}
]
```

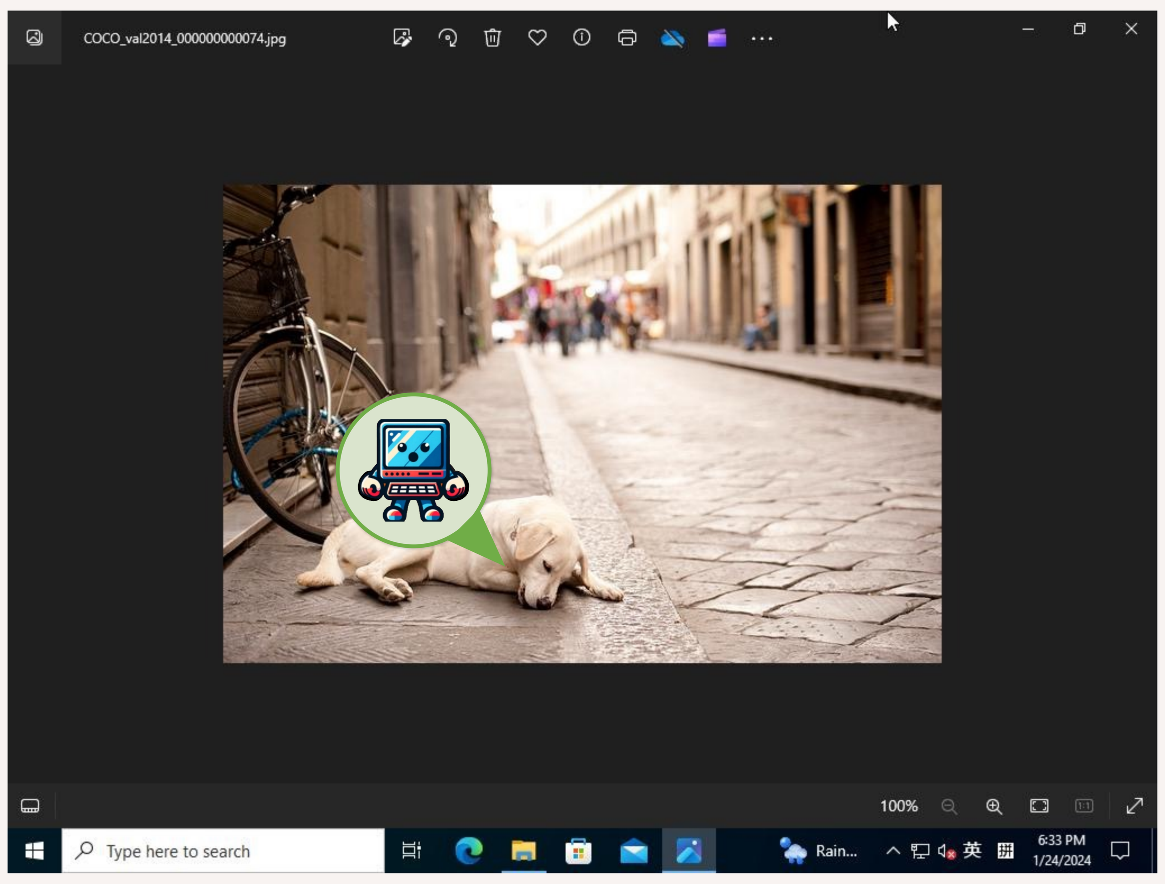


**Subtask:** Please click the dog in the picture

**ScreenAgent(Acting Phase):**
To complete "Please click the dog in the picture", I need to finish the current_task "Click the dog" by this action:
```json
[
  {"action_type":"MouseAction", "mouse_action_type":"click",
"mouse_button":"left", "mouse_position":{"width":449,"height":495}}
]
```

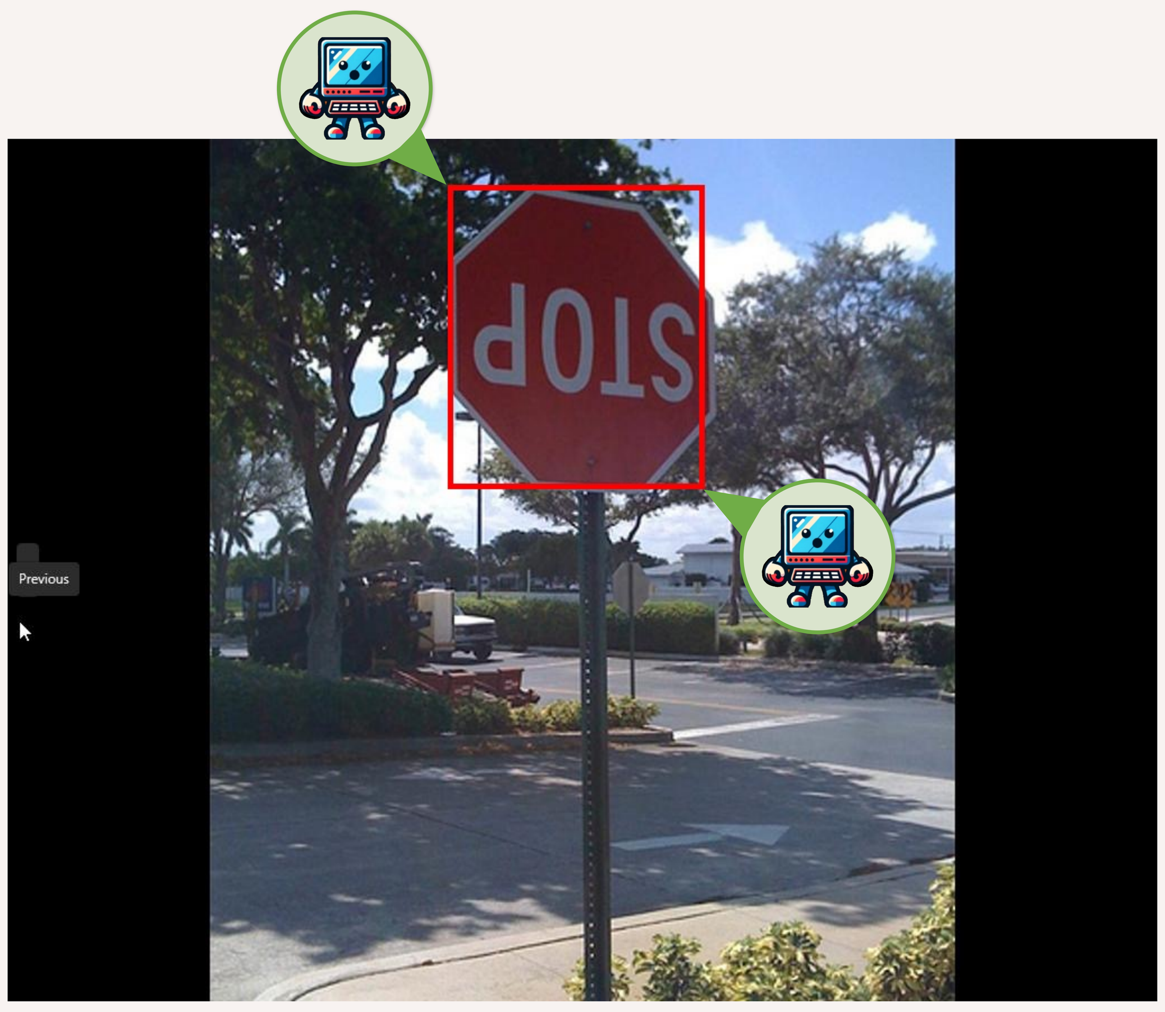


**Subtask:** drag draw a box of stop sign

**ScreenAgent(Acting Phase):**
To finish drag draw a box of stop sign, i will click UI element by this action:
```json
[
  {"action_type":"MouseAction","mouse_action_type":"move","mouse_posi
tion":{"width":393,"height":42}},
  {"action_type":"MouseAction","mouse_action_type":"drag","mouse_butt
on":"left","mouse_position":{"width":619,"height":310}}
]
```

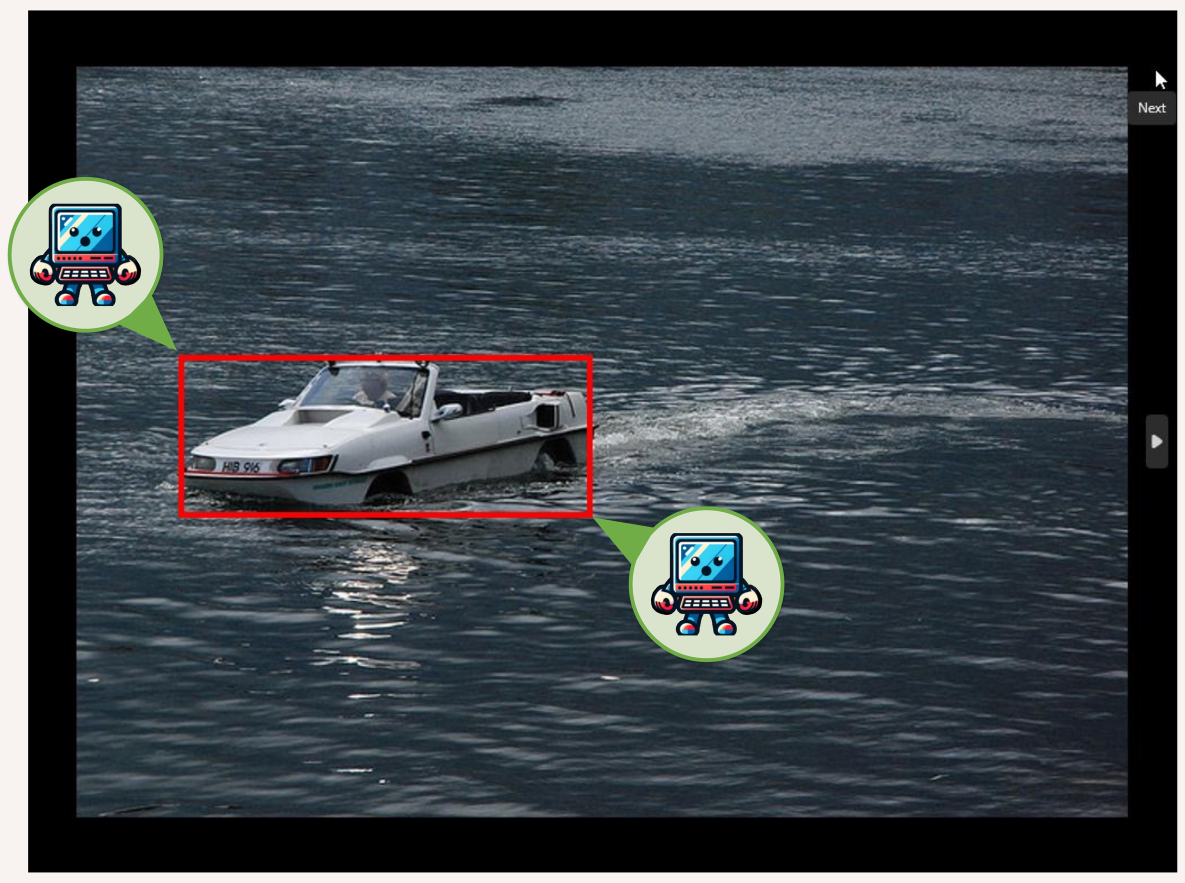


**Subtask:** drag draw a box of boat

**ScreenAgent(Acting Phase):**
To finish "drag draw a box of boat", I need to finish the current task "drag draw a box of boat" by this action:
```json
[
  {"action_type":"MouseAction","mouse_action_type":"move","mouse_posi
tion":{"width":135,"height":308}},
  {"action_type":"MouseAction","mouse_action_type":"drag","mouse_butt
on":"left","mouse_position":{"width":500,"height":449}}
]
```

# User:Watch a tutorial video on seated rowing

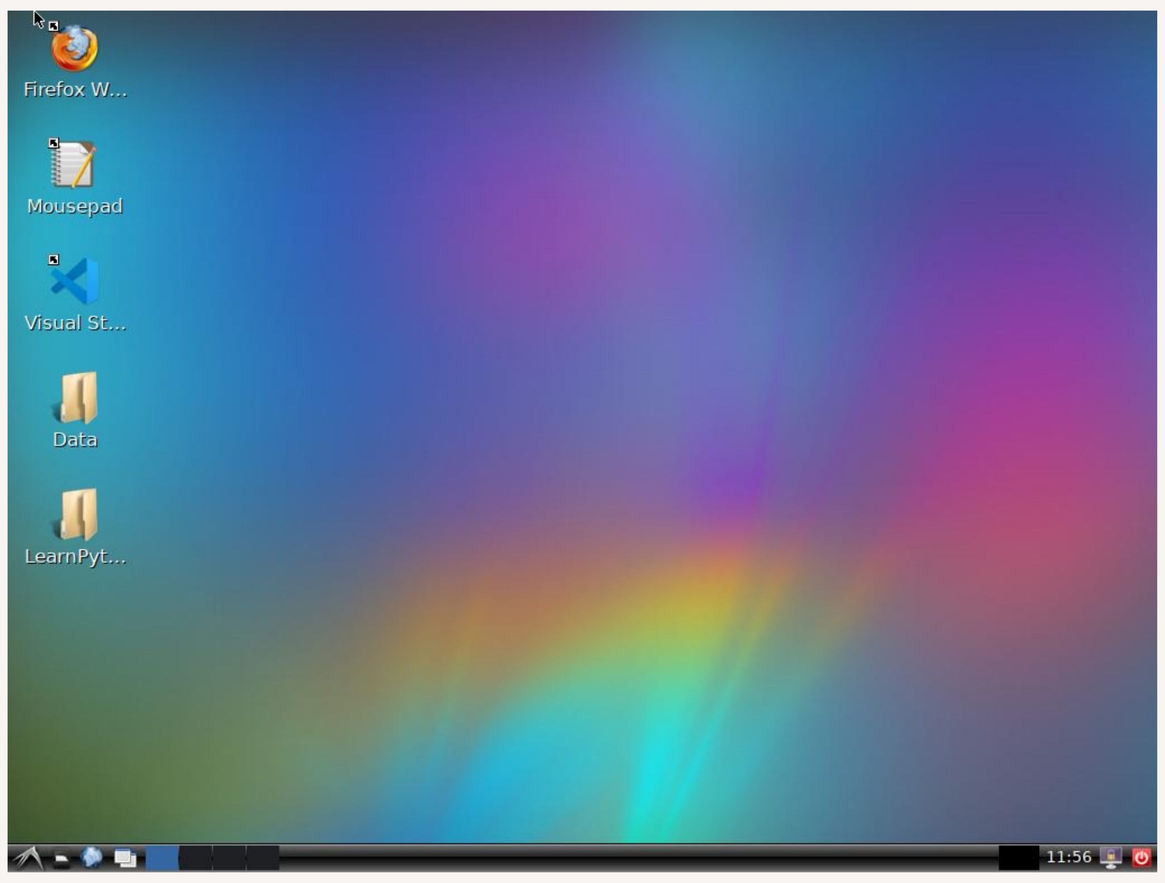

**Screen Agent(Planning Phase):**

```json
[
  {"action_type":"PlanAction","element":"Open browser"},
  {"action_type":"PlanAction","element":"Enter the video website URL in the browser address bar"},
  {"action_type":"PlanAction","element":"Enter the search term    "seated rowing tutorial" in the video website search box"},
  {"action_type ":"PlanAction","element":"Find the appropriate seated rowing tutorial video in the search results and watch it"}
]
```

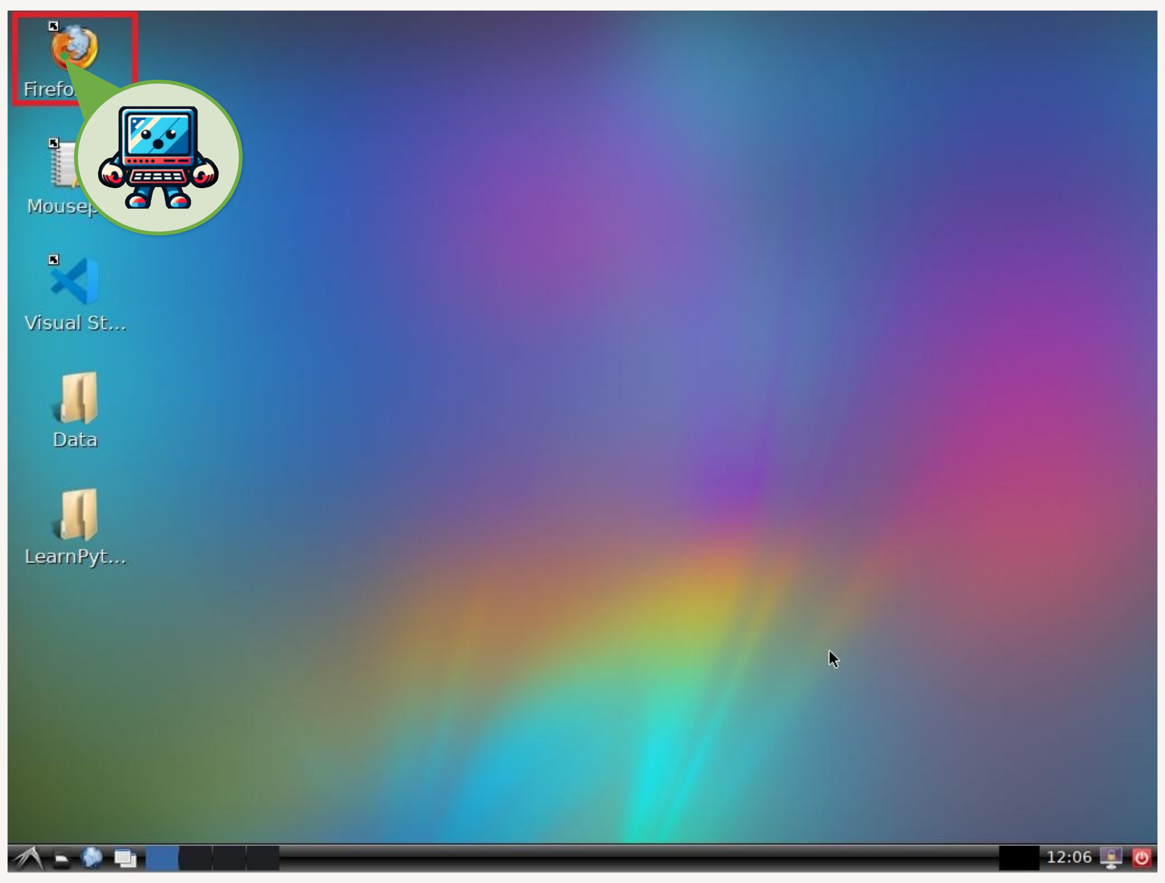

**Subtask:**Open browser

**Screen Agent(Acting Phase):**

According to the screen image provided, the Firefox Web Browser icon is located in the upper left corner of the desktop. To execute the subtask "Double-click on the Firefox Web Browser icon to open it.",the following JSON action sequence will be performed:

```json
[
  {"action_type":"MouseAction","mouse_action_type":"double_click“,"mouse_button":"left","mouse_position":{"width":50,"height":40}}
]
```

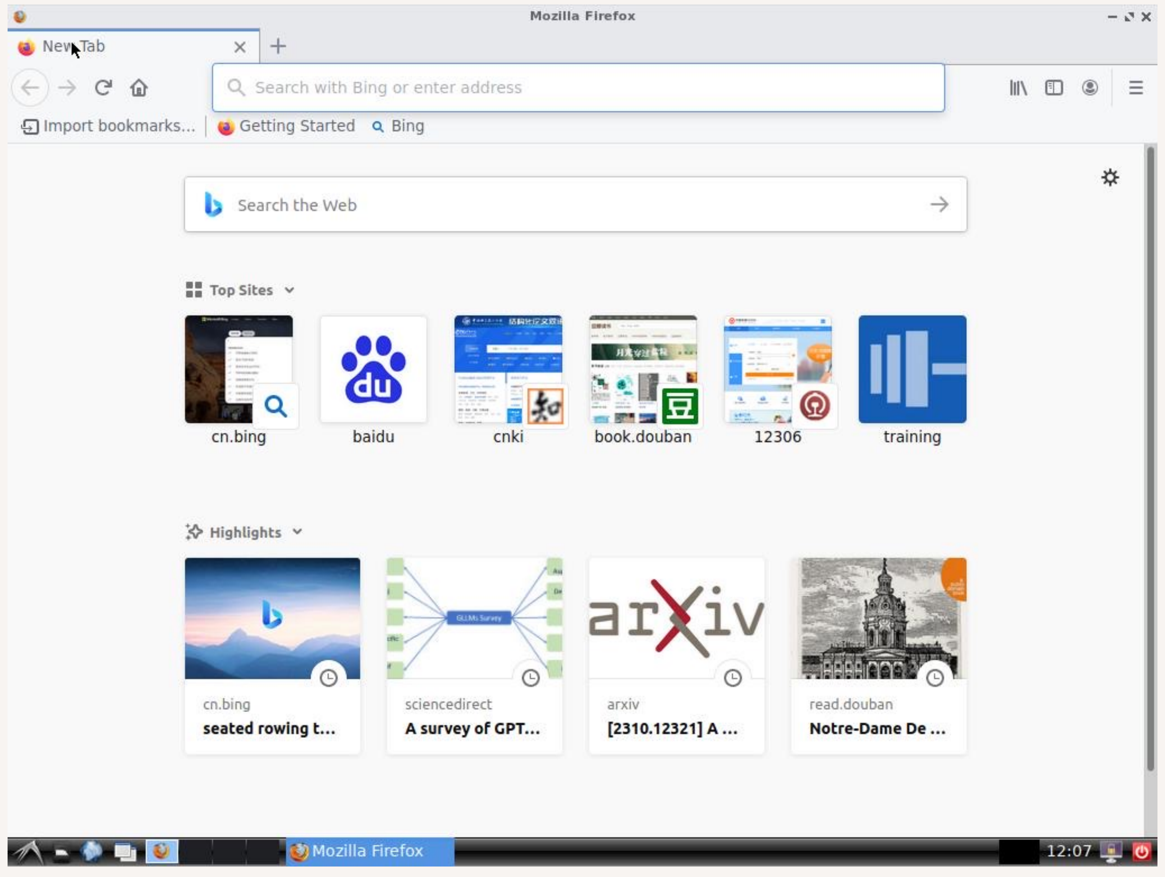


**Subtask:**Open browser

**Screen Agent(Reflecting Phase):**

```json
[
  {
    "action_type": "EvaluateSubTaskAction",
    "situation": "sub_task_success“
  }
]
```

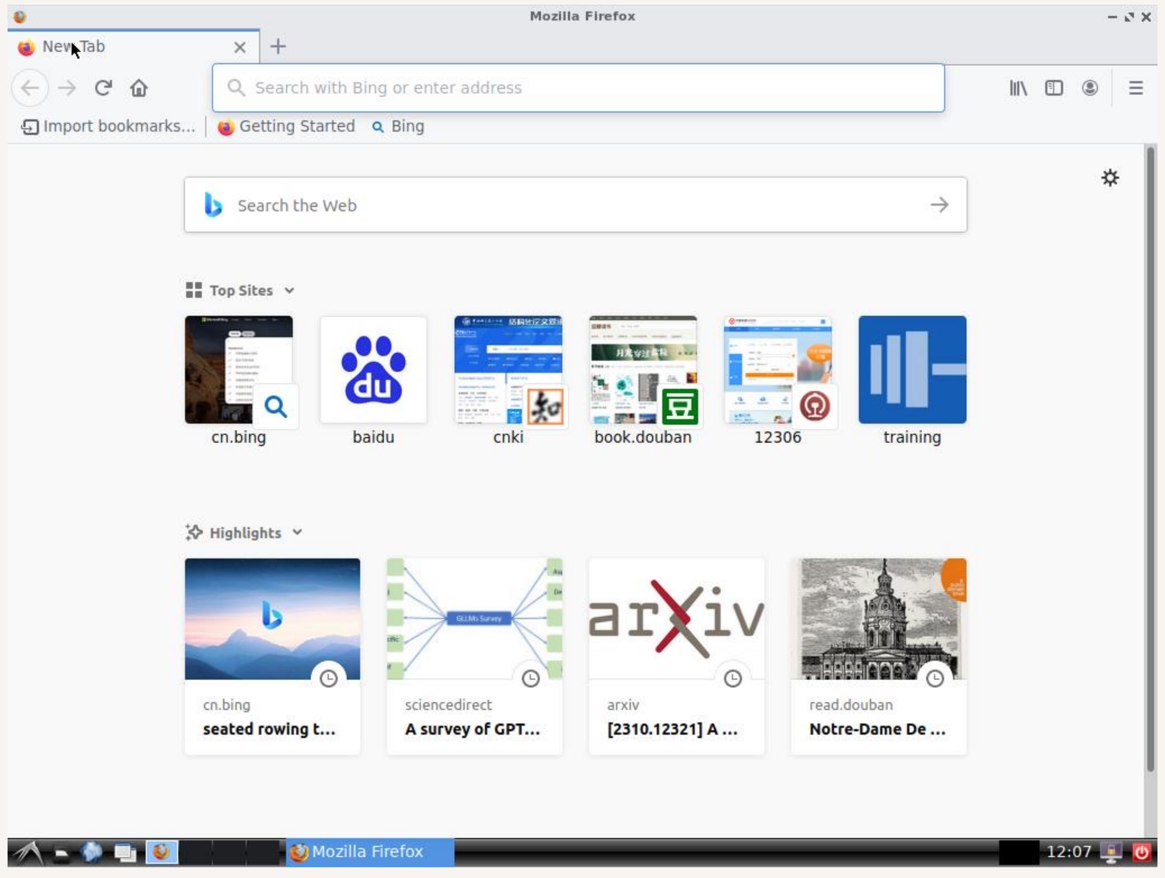


**Subtask:**Enter the video website URL in the browser address bar

**Screen Agent(Acting Phase):**

To complete the subtask  "Go to the bilibili website ", we need to perform the following operations:

```json
[
  {"action_type":"KeyboardAction","keyboard_action_type":"text", "keyboard_text":"www.bilibili.com"},
  {"action_type":"KeyboardAction","keyboard_action_type":"press", "keyboard_key":"Return"}
]
```

This will open the browser and navigate to the bilibili website.

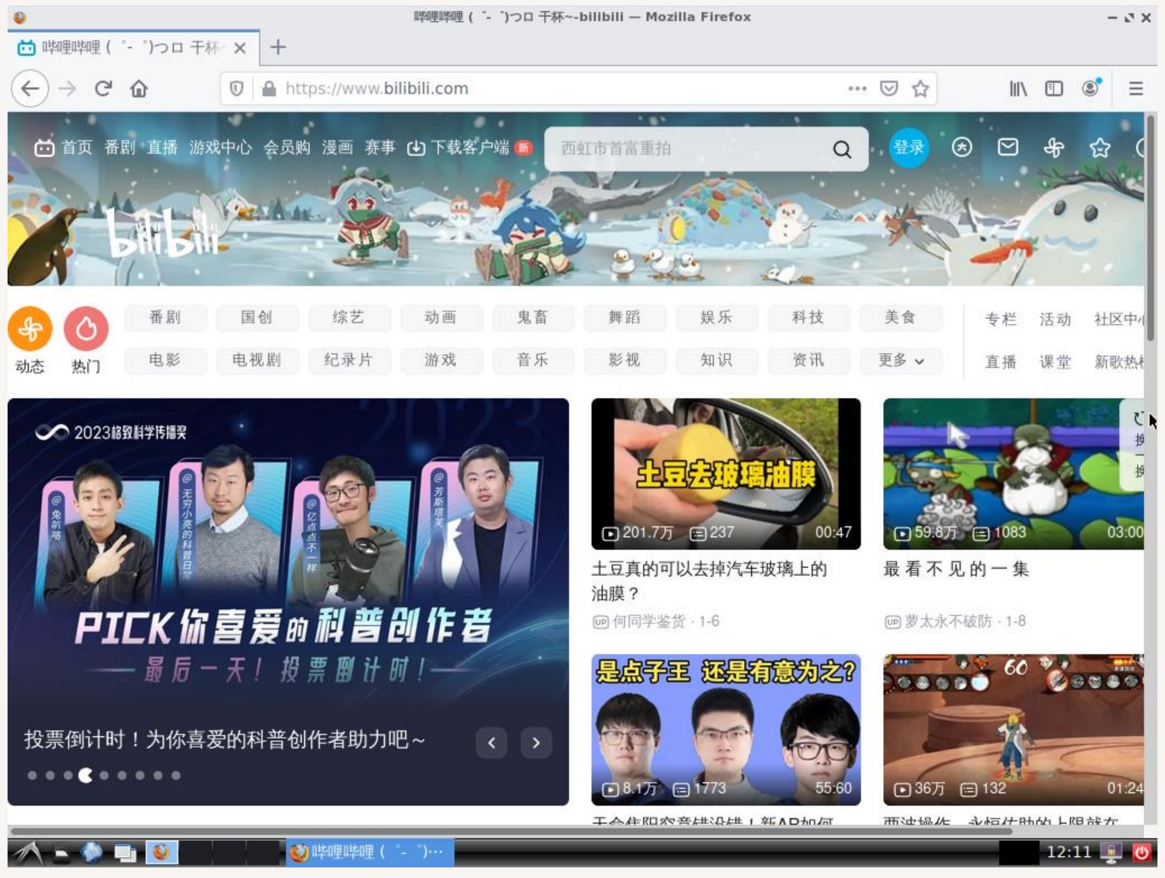


**Subtask:**Enter the video website URL in the browser address bar

**Screen Agent(Reflecting Phase):**

```json
[
  {
    "action_type":"EvaluateSubTaskAction",
    "situation": "sub_task_success“
  }
]
```

You can see that the bilibili website has been opened in the browser window, and you can continue to perform the next subtask.

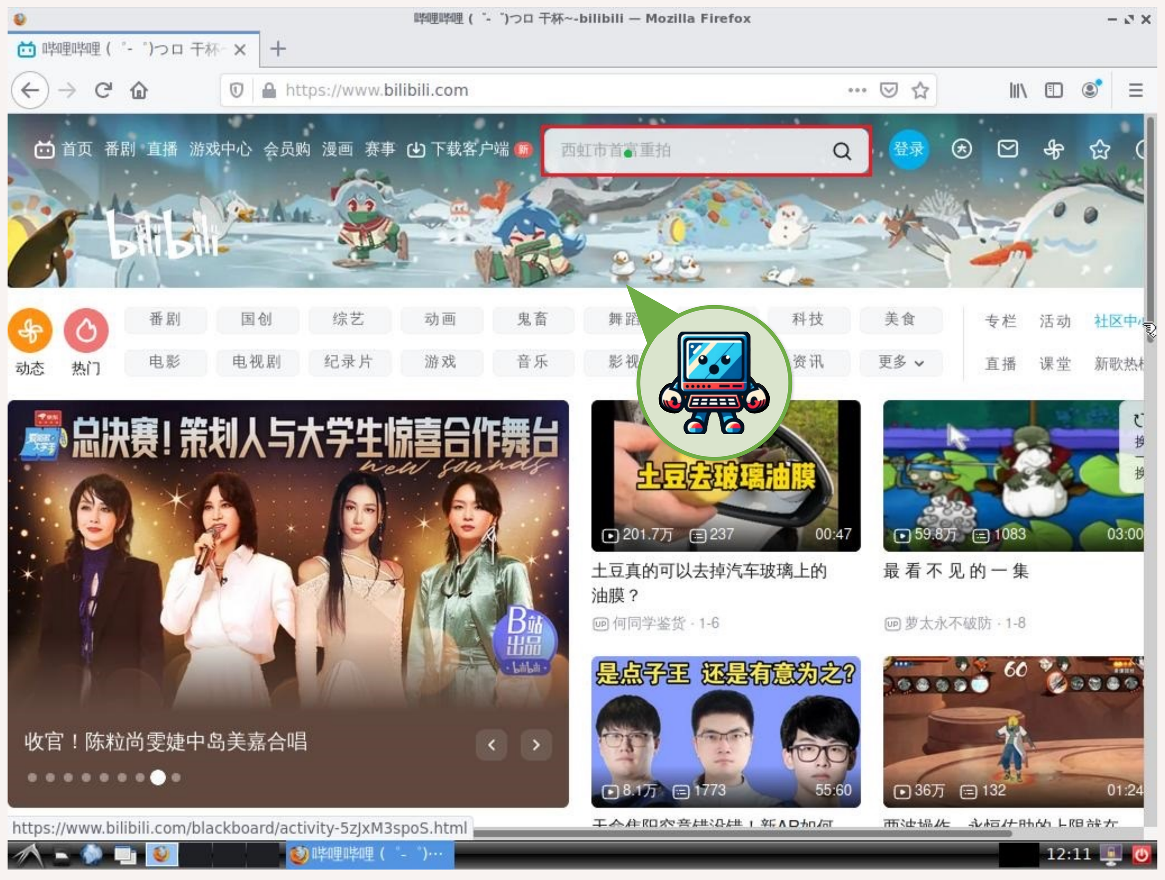

**Subtask:**Enter the search term "seated rowing tutorial" in the video website search box

**Screen Agent(Acting Phase):**

According to the screenshot you provided, the search box is located in the upper central area of the screen, and the text "seated rowing tutorial " is entered in the search box. Now, we need to perform the following actions to complete the subtask of "Enter 'seated rowing tutorial' in the search field ":

```json
[
  {"action_type":"MouseAction","mouse_action_type":"click","mouse_button":"left","mouse_position":{"width":552,"height":130}},
  {"action_type":"KeyboardAction","keyboard_action_type":"text","keyboard_text":"seated rowing tutorial"},
  {"action_type":"KeyboardAction","keyboard_action_type":"press","keyboard_key":"Return"}
]
```

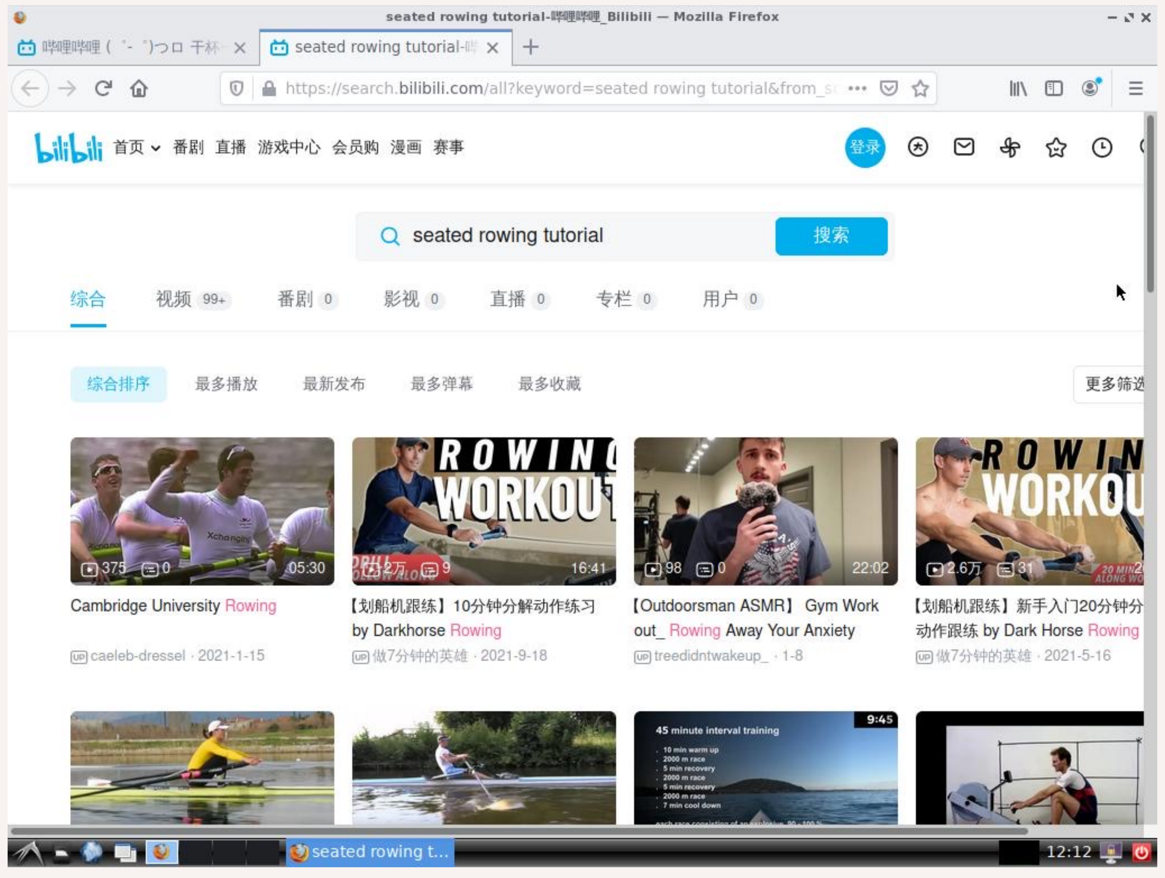

**Subtask:**Enter the search term "seated rowing tutorial" in the video website search box

**Screen Agent(Reflecting Phase):**

```json
[
  {
    "action_type": "EvaluateSubTaskAction",
    "situation": "sub_task_success“
  }
]
```

You can see that the search field has been filled with 'seated rowing tutorial', and the next step can be carried out.

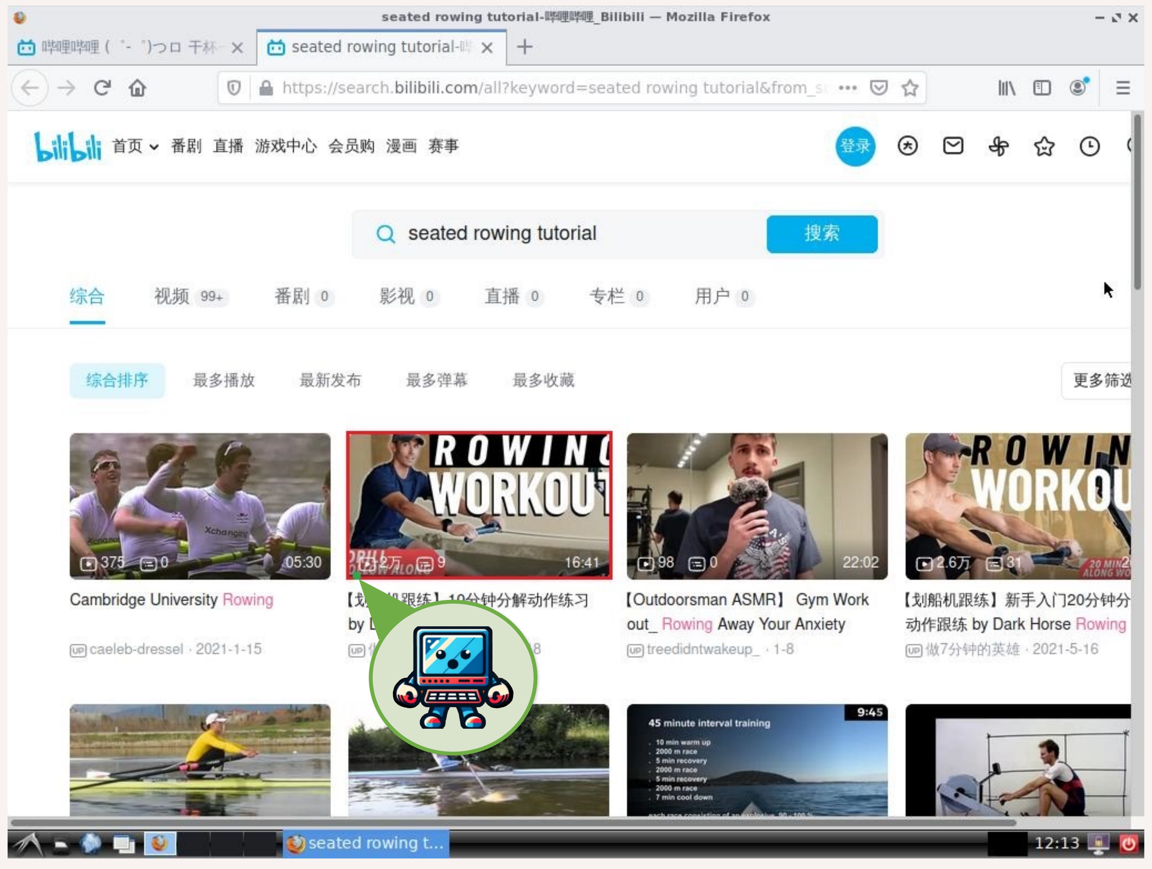

**Subtask:**Find the appropriate seated rowing tutorial video in the search results and watch it

**Screen Agent(Acting Phase):**

According to the screenshot, we can see that the search results are displayed on the screen, and the first video is a video about seated rowing. Therefore, we need to perform the following actions to click on the video:

```json
[
  {"action_type":"MouseAction","mouse_action_type":"click","mouse_button":"left","mouse_position":{"width":315,"height":513}}
]
```

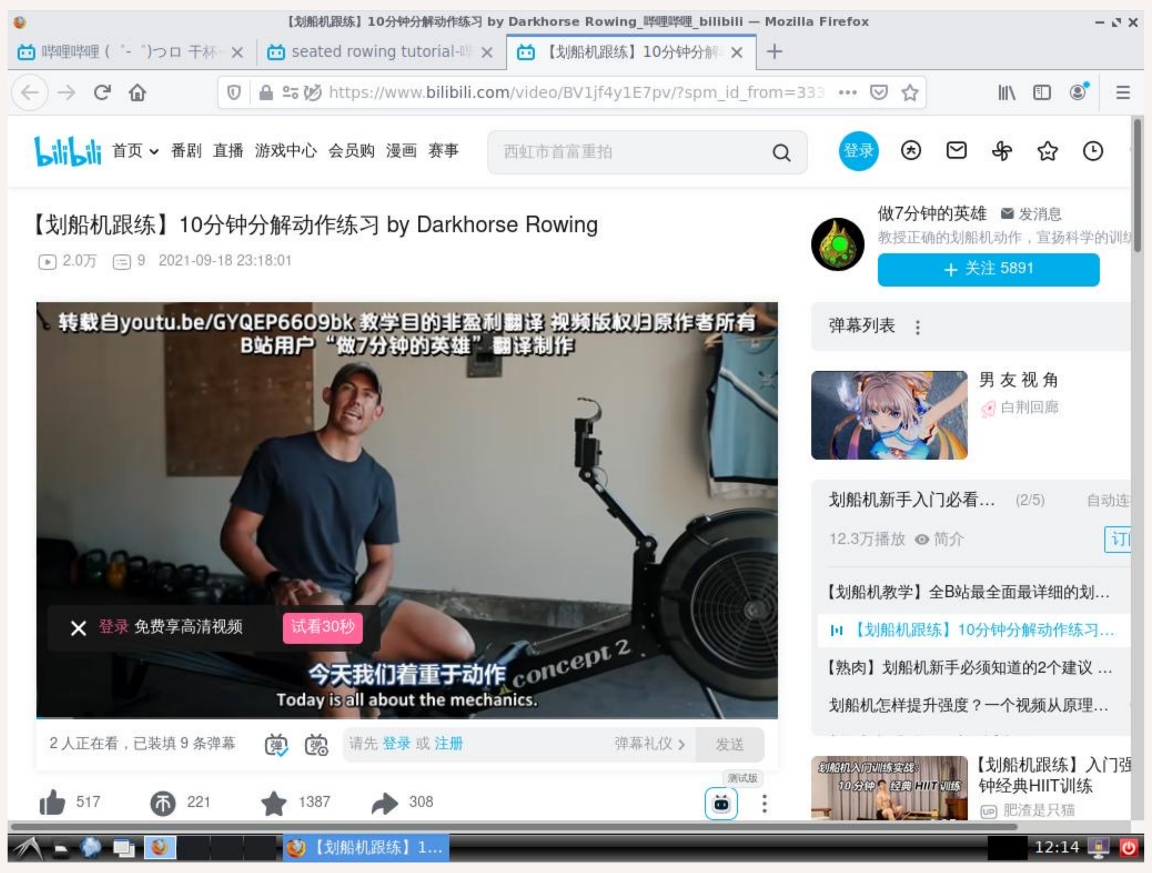

**Subtask:**Find the appropriate seated rowing tutorial video in the search results and watch it

**Screen Agent(Reflecting Phase):**

```json
[
  {
    "action_type":"EvaluateSubTaskAction",
    "situation": "sub_task_success“
  }
]
```

You can see that the video is playing.
